# Supplementary material for: Dislocations and the enhancement of superconductivity in odd-parity superconductor Sr$_2$RuO$_4$
Source: arXiv:1205.3250 source file (2012-05-15)
Supplement: Supplementary file 1 [file Supplemental_Material.pdf]

# Supplemental Material

# Dislocations and the enhancement of superconductivity in odd-parity superconductor $Sr_2RuO_4$

Y. A. Ying, N. E. Staley, Y. Xin, K. Sun, X. Cai, D. Fobes, T. Liu, Z. Q. Mao, and Y. Liu

## 1. Phenomenological theory

Following Eq. (2) of the main text, the transition temperature for the symmetry broken homogeneous system can be obtained by the eigenvalues $\lambda_+$ and $\lambda_-$ of the coefficients of the quadratic terms, which leads to

$$\lambda_\pm = a + m_+ \pm \sqrt{m_-^2 + |\mu|^2} \qquad \text{S (1)}$$

where $m_\pm=(m_1 \pm m_2)/2$. The higher transition temperature $T_{ch}$ can be obtained by demanding $\lambda_- = 0$, which reads

$$T_{ch} = T_{c0} + \frac{1}{\alpha}(\sqrt{m_-^2 + |\mu|^2} - m_+) \qquad \text{S (2)}$$

The term associated with $m_+$ may either enhance or suppress $T_{ch}$, depending on its sign. The square root term, which measures the anisotropy between the $x$ and $y$ component of the order parameter, always enhances $T_{ch}$. Since $m_1$, $m_2$ and $\mu$ are proportional to the strength of the lattice distortions, we may treat $m_1$ and $m_2$ as a linear function of $\mu$. We found that in most of the parameter space, an enhancement in $T_{ch}$ can be obtained [Fig. 1(c) of the main text].

To solve the linearized Ginzburg-Landau equations on the stripe, we adopt constrains for $K_j$ used in Ref. 18, $K_1/3 = K_2 = K_3 = K_4 >> K_5$. In the geometry we consider, the problem can be simplified into a one dimensional problem by ignoring the variations along the $y$ and $z$ axis. To examine the onset $T_c$, we consider the linearized Ginzburg-Landau equations derived from Eq. (1) of the main text

$$K_1\partial_x^2\eta_x - a\eta_x = 0 \qquad \text{S (3)}$$

$$K_2\partial_x^2\eta_y - a\eta_y = 0 \qquad \text{S (4)}$$

for $x \neq 0$. For $x = 0$, we assume a fully transparent boundary, at which the solutions have to be continuous. Meanwhile, the solutions satisfy the boundary conditions derived from Eq. (4) of the main text

$$K_1\partial_x\eta_x|_{x=0+} - K_1\partial_x\eta_x|_{x=0-} - \alpha d(T - T_{ch})\eta_x = 0 \qquad \text{S (5)}$$

$$K_2\partial_x\eta_y|_{x=0+} - K_2\partial_x\eta_y|_{x=0-} - \alpha d(T - T_{ch})\eta_y = 0 \qquad \text{S (6)}$$

The solutions for temperatures above $T_{c0}$ have the following forms

$$\eta_x = \eta_{x0}\exp(-x/\xi_1) \quad \text{for } x > 0 \qquad \text{S (7)}$$

$$\eta_x = \eta_{x0}\exp(x/\xi_1) \quad \text{for } x < 0 \qquad \text{S (8)}$$

where $\xi_1(T) = (K_1/|a|)^{1/2}$.

$\eta_y = \eta_{y0}\exp(-x/\xi_2)$ for x > 0 S (9)

$\eta_y = \eta_{y0}\exp(x/\xi_2)$ for x < 0 S (10)

where $\xi_2(T) = (K_2/|a|)^{1/2}$. Matching the boundary conditions S (5) and S (6), we obtain the following equations

$$2\sqrt{K_1\alpha(T-T_{c0})} + \alpha d(T-T_{ch}) = 0 \quad \text{S (11)}$$

$$2\sqrt{K_2\alpha(T-T_{c0})} + \alpha d(T-T_{ch}) = 0 \quad \text{S (12)}$$

Note that if $T_{ch} > T_{c0}$, we always have a solution $T_c$ such that $T_{ch} > T_c > T_{c0}$. Meanwhile, because $K_1/3 = K_2$, Eq. S (12) gives a higher instability temperature, indicating that the $y$-component becomes non-zero first.

To obtain the spatial dependence of the order parameters, we numerically solve the Ginzburg-Landau equations by taking the phenomenological parameters $2b_1 = 3b_2 = -3b_3 = 0.4\alpha$, $T_{ch} = 3$ K, $K_1/\alpha T_{c0} = 3K_2/\alpha T_{c0} = 1$, the same as those used in Ref. 18. We expand the $\delta$-function in Eq. (4) of the main text into a Gaussian function. The Ginzburg-Landau equations then read

$$K_1\partial_x^2\eta_x - \alpha(T-T_{c0})\eta_x - \frac{\alpha(T-T_{ch})}{\sqrt{2\pi}}e^{-\frac{x^2}{2d^2}}\eta_x - 2b_1(\eta_x^2+\eta_y^2)\eta_x = 0 \quad \text{S (13)}$$

$$K_2\partial_x^2\eta_y - \alpha(T-T_{c0})\eta_y - \frac{\alpha(T-T_{ch})}{\sqrt{2\pi}}e^{-\frac{x^2}{2d^2}}\eta_y - 2b_1(\eta_x^2+\eta_y^2)\eta_y = 0 \quad \text{S (14)}$$

where $K_1/\alpha T_{c0} = 3K_2/\alpha T_{c0} = 1$, $d = 1.41(K_2/\alpha T_{c0})^{1/2} = 0.82$, giving rise to $T_c = 1.9$ K. When $x$ goes to infinite, the solutions decay to zero for $T > 1.5$ K and approach a constant of $\eta_x = \eta_y = (-a/4b_1)^{1/2}$ for $T < 1.5$ K. The results were plotted in Fig. 1(d) of the main text.

## 2. Materials and measurements

We started with a batch of easily cleavable bulk single crystals of $Sr_2RuO_4$. This batch was grown by a floating zone method with the starting material slightly less Ru rich than usual. Because of the high vapor pressure of $RuO_2$, excess Ru needs to be added in order to form a crystal with the correct atomic ratio. In the crystal we used, 10% excess Ru was added. The bulk onset $T_c$ was found to be 1.35 K, lower than the optimal $T_c$ (1.5 K) of $Sr_2RuO_4$ (Supplemental Material Fig. 1). The superconducting transition in the bulk crystal was found to be broad, with a zero-resistance $T_c$ of 0.71 K, suggesting the presence of inhomogeneity.

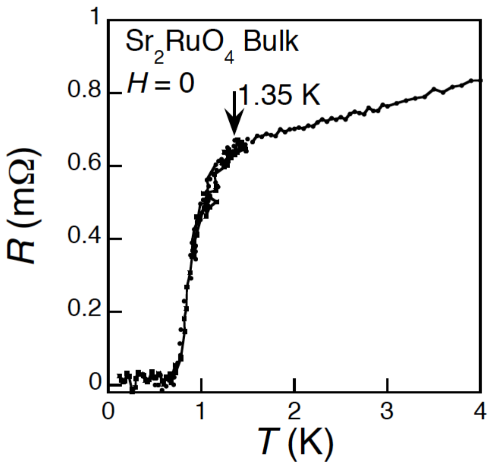


Supplemental Material FIG. 1. Zero-field sample resistance plotted as a function of temperature for a bulk piece of $Sr_2RuO_4$ crystal.

To make TEM samples of $Sr_2RuO_4$ crystal flakes, the bulk $Sr_2RuO_4$ crystal was sonicated in methanol. Droplets containing tiny flakes of $Sr_2RuO_4$ crystals were dripped onto a TEM grid with carbon membrane. After the methanol dried, the $Sr_2RuO_4$ crystals remained on the carbon membrane. Selected thin pieces of such crystals were studied by TEM. Some crystals are free of Ru microdomains and dislocations (Supplemental Material Fig. 2). On the other hand, small crystals with Ru microdomains on the edge and a large amount of dislocation lines were also observed (Fig. 1a of the main text). It is interesting that two types of small $Sr_2RuO_4$ crystals, with or without dislocations, can be obtained from the same bulk crystal whose onset $T_c$ is 1.35 K.

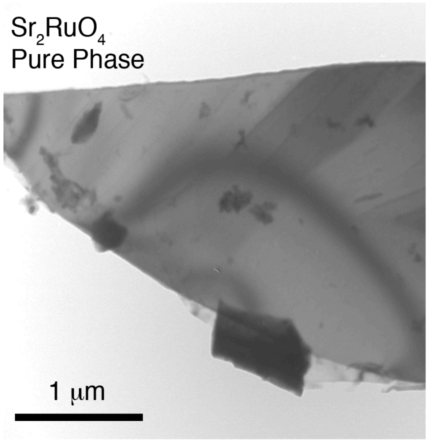


Supplemental Material FIG. 2. TEM image of a $Sr_2RuO_4$ crystal flake with neither Ru nor dislocations.

To fabricate devices for transport measurements, flat small crystals of slightly larger sizes

than those used in the above TEM studies were obtained by mechanically cleaving the bulk crystal. Standard four-point transport devices were made on regularly shaped small crystals with a typical dimension of 30 μm × 10 μm × 500 nm. An SEM image of Sample 2 mentioned in the main text can be seen in Supplemental Material Fig. 3. Low temperature dc measurements were performed in a $^3$He refrigerator with a base temperature of 0.35 K. All leads entering the cryostat are shielded and filtered by low-pass RC filters with a 3 dB cut-off frequency of 600 kHz. After carrying out electric transport measurements at low temperatures, the crystal flake of Sample 1 was further transferred onto a TEM grid using the standard tool of a tungsten tip.

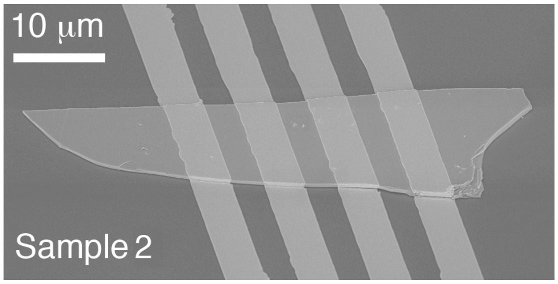


Supplemental Material FIG. 3. SEM image of Sample 2.

The magnetic field dependence of $J_c$ was found to behave similarly in both types of crystals for field parallel to the in-plane direction. For a *c* axis field, they also show very similar behavior (Supplemental Material Fig. 4), consistent with the collective pinning theory for intermediate field values. The $J_c(H)$ for *c* axis field supports the fact that the vortex pinning is not enhanced by the presence of dislocations and/or tiny Ru microdomains if the latter turns out to be responsible for the observed $T_c$ enhancement.

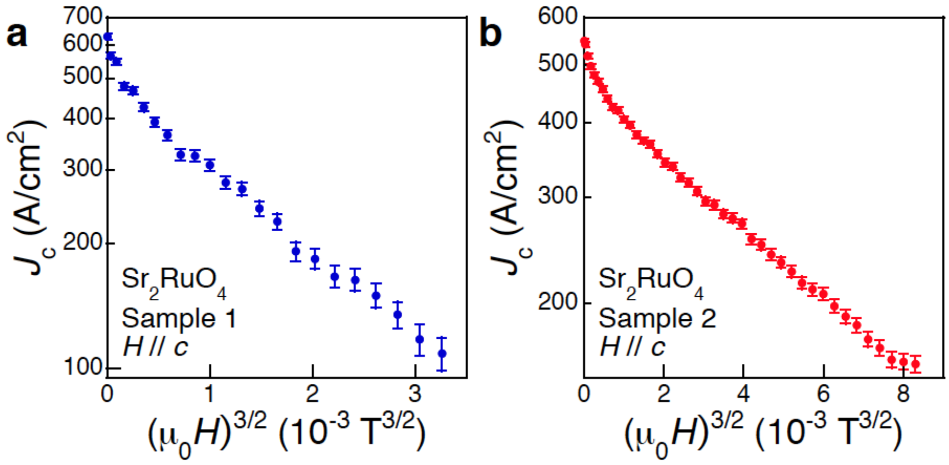


Supplemental Material FIG. 4. $J_c$ plotted logarithmically as a function of $H^{3/2}$ for field perpendicular to the in-plane direction for (a) Sample 1 with enhanced $T_c$ and (b) Pure phase Sample 2.
